# Supplementary material for: Metadata-based Multi-Task Bandits with Bayesian Hierarchical Models
Source: arXiv:2108.06422 source file (2021-08-13)
Supplement: Supplementary file 1 [file Additional_Related_Work.tex]

\section{Additional Related Work}\label{sec:appendix_additional_related_work}
In this section, we compare this paper with additional related works. 
To begin with, we note that there are several terms used in the literature for problems concerned with multiple tasks, which is often a source of confusion. 
Based on  \cite{hospedales2020meta}, 
\textit{meta learning} assumes tasks are drawn from a distribution and aims to maximize the average performance over this task distribution (\textit{meta-objective}); 
\textit{transfer learning} uses data from finished tasks to improve the performance on a new task, and typically focuses on the single-task objective, although the viewpoint of meta learning can be applied to achieve this goal (as in the sequential setting of our work); 
\textit{multi-task learning} aims to jointly learn a few tasks, where typically the number of tasks is fixed and the meta-objective is not adopted, although the viewpoint of meta learning can be applied in these problems as well (as in the concurrent setting of our work). 
There are often some overlaps between these concepts. 
In this work, we adopt the task distribution viewpoint as well as the meta-objective \cite{hospedales2020meta}, which are naturally related with our hierarchical Bayesian framework, allows us to model heterogeneity, and enables knowledge sharing via constructing informative priors. 
We refer to our problem as multi-task bandits to focus on the fact that there are multiple tasks, since our methodology is applicable to the sequential setting (transfer learning), the concurrent setting (multi-task learning), and even more complex settings. 
% Continual learning (CL) Continual or lifelong learning

% Low-rank bandits. is an extention
According to the taxonomy developed in \cite{zhang2017survey}, multi-task algorithms can be classified into the feature learning approach, low-rank approach, task clustering approach, task relation learning approach, and decomposition approach. 
In the bandit literature, \cite{yang2021impact} considers that one interacts with multiple linear bandit
tasks concurrently and the coefficient vectors of these tasks share the same low-dimensional space, and hence belongs to the feature learning approach; 
\cite{kveton2017stochastic} studies finding the maximum entry of a low-rank matrix in a bandit manner and \cite{jun2019bilinear} assumes the coefficient matrix of a bilinear bandit problem is low-rank, and hence they belong to the low-rank approach; 
clustering of bandits \citep{gentile2014online, li2016collaborative} and latent bandits \citep{hong2020latent, hong2020non} assume there is a perfect clustered structure, and hence they belong  to the task clustering approach. 
In contrast to these papers, our work belongs to the relation learning approach, which aims to learn the task relations from data by assuming some probabilistic model or applying some penalty function. 
Our approach provides nice interpretability and is flexible with arguably less strict assumptions.  
In particular, to the best of our knowledge, this is the \textit{first} work that can leverage the task-specific metadata in multi-task bandits, which is an important information source that none of the existing methods can utilize. 
Although we focus on MAB in the main text, the idea of utilizing metadata is generally applicable. 
We discuss its extensions to linear bandits and clustering of bandits in Appendix \ref{sec:extension_contextual}.

Besides, similar with meta MAB, there are also several works on meta linear bandits. 
Meta linear bandits studies the problem where the coefficients of multiple linear bandit tasks are close \citep{multilinear} or are drawn from one prior distribution \citep{metapricing, tomkins2019intelligent, cella2020meta}. 
% IP in the appendix. % random coeffcient model % share some similar technical tools 
Therefore, these works focus on a different problem from ours and they also did not model the task relations with metadata. 
In addition, \cite{ortega2019meta} proposes a sequential strategy for meta bandits, but as noted in \cite{hsu2019empirical}, no efficient algorithm has been proposed. 
Lastly, we note that there are two papers \cite{deshmukh2017multi, krause2011contextual} applying multi-task learning to share information across multiple arms of a single task, and hence they have a totally different focus from ours. 

% metadata and BHM is main.
% : transfer RL survey. 
% In the main text, we focus on the literature on bandits. 
% at a high level, 
Our bandit problem is certainly related to Reinforcement Learning (RL). 
In recent years, there is a surge of interest in multi-task RL, transfer RL, and meta RL. 
See \cite{zhu2020transfer} and \cite{vithayathil2020survey} for some recent surveys. 
Among the existing works, 
\cite{wilson2007multi, lazaric2010bayesian, grant2018recasting} consider applying Bayesian hierarchical model to multi-task/meta RL. 
However, none of these works can utilize the metadata, which is an important and ubiquitous information source. 
In the concurrent work \cite{sodhani2021multi}, the authors, for the first time, consider using metadata in multi-task reinforcement learning to infer the appropriate state representation for each task. 
They consider a finite set of state encoders, design a special-purpose neural network, and train the whole pipeline end-to-end. 
In contrast, 
we study MAB, allow infinite number of task instances, aim to learn the average reward of each task instead of state representation,  design a unified Bayesian Hierarchical model framework for this problem, and establish theoretical guarantees. 
Therefore, although both work consider similar types of side information (i.e., metadata), the problem and methodology are fundamentally different.

Finally, we would like to further compare our setup with CMAB, and discuss the limitations of adopting CMAB in our problem. 
In the standard contextual MAB setup, we assume $\Mean(R_{i,t}|S_{i,t} = s, A_{i,t} = a) = g(s, a;\gamma)$ for some function $g$, where $S_{i,t}$ is the context. 
Therefore, it already allows the randomness of $R_{i,t}$. 
In our setup,  by regarding the metadata as "contexts" and neglecting the task identities, the relationship is equal to $\Mean(R_{i,t}|\vx_{i} = \vx, A_{i,t} = a) = g(\vx, a;\gamma)$, where we note that the expectation is taken over all tasks with metadata $\vx$. 
This implies that for all tasks with the same metadata, the decision rule will be always the same, no matter what their action-reward history is. 
Instead, our setup adds another layer to allow variations of $\vr_i$ conditional on $\vx_i$. 
In another word, we utilize the predictive power of $\vx_i$ but does not assume $\vr_i$ can be fully determined by it. 
% by neglecting the task identities and regarding the metadata as "contexts". % static metadata
% and hence it is reasonable to assume $\vr_i = f(\vx_i)$
% Recall that $\vr_i$ is the expected reward vector for all arms

% warm-starting bandit / offline data: the same bandit task
% collaborative filtering: metaTS

% ,  assumes such a clustered structure has been learned from logged data. 
% Multi-task Linear Bandits: sequential, epsilon
