# Supplementary material for: Metadata-based Multi-Task Bandits with Bayesian Hierarchical Models
Source: arXiv:2108.06422 source file (2021-08-13)
Supplement: Supplementary file 4 [file Additional_Results.tex]

\section{Additional Experiment Results}\label{sec:appendix_addi_numerical_results}

\subsection{Robustness to model misspecifications}\label{sec:appendix_robustness}
To allow efficient information sharing, we make a model assumption that $\vr_i | \vx_i, \vthe \sim f(\vr_i | \vx_i, \vthe), \forall i \in [N]$. 
When this model is correctly specified, we have shown superior theoretical and numerical performance of {\name}. 
However, we acknowledge that all models can be misspecifed. 
Intuitively, the model is used to pool information to provide an informative prior. 
As long as the learned prior is not significantly worse than a manually specified one, the performance would be comparable; and when the prior contains more information, we can attain a lower regret. 

We empirically investigate the robustness of {\name} in this section. 
We focus on the Gaussian bandits case under the concurrent setting. 
Findings under the other settings are largely the same and hence omitted. 
Specifically, 
instead of generating data according to $\vr_i = \vPhi_{i}\vthe + \vdelta_i$, we consider the data generation process $\vr_i = (1 - \lambda) cos(c\vPhi_{i}\vthe)/c + \lambda \vPhi_{i}\vthe  + \vdelta_i$, where $cos$ applies the cosine function to each entry, 
c is a normalization constant such that the entries of $\vPhi_{i}\vthe$ are all in $[-\pi/2,\pi/2]$, 
and $\lambda \in [0,1]$ controls the degree of misspecification. 
When $\lambda = 1$, we are considering the LMM; while when $\lambda = 0$, the metadata  provides few  information through such a linear form. 

In results reported in Figure \ref{fig:simu_Gaussian_robustness_concurrent}, we observe that {\name} is fairly robust to model misspecifications. 
When $\lambda = 1/2$ or $3/4$, that is, when there exists mild or moderate misspecification, {\name} still yields much lower regrets than individual-TS and meta-TS. 
When $\lambda = 1/4$, the performance of {\name} becomes comparable with individual-TS and meta-TS. 
Only when $\lambda = 0$, that is, the metadata are useless through a linear form, {\name} shows slightly higher regret in the initial period due to the additionally introduced variance. 
As expected, linear-TS and OSFA both severely suffer from the bias. 
Notably, in all cases, {\name} always yields the desired sublinear Bayes regret in $T$, as expected. 
Therefore, it shows that, even when the model is severely misspecified, the cost would be acceptable.

\begin{figure}[h]
     \centering
     \begin{subfigure}[b]{\textwidth}
         \centering
         \includegraphics[width=\textwidth]{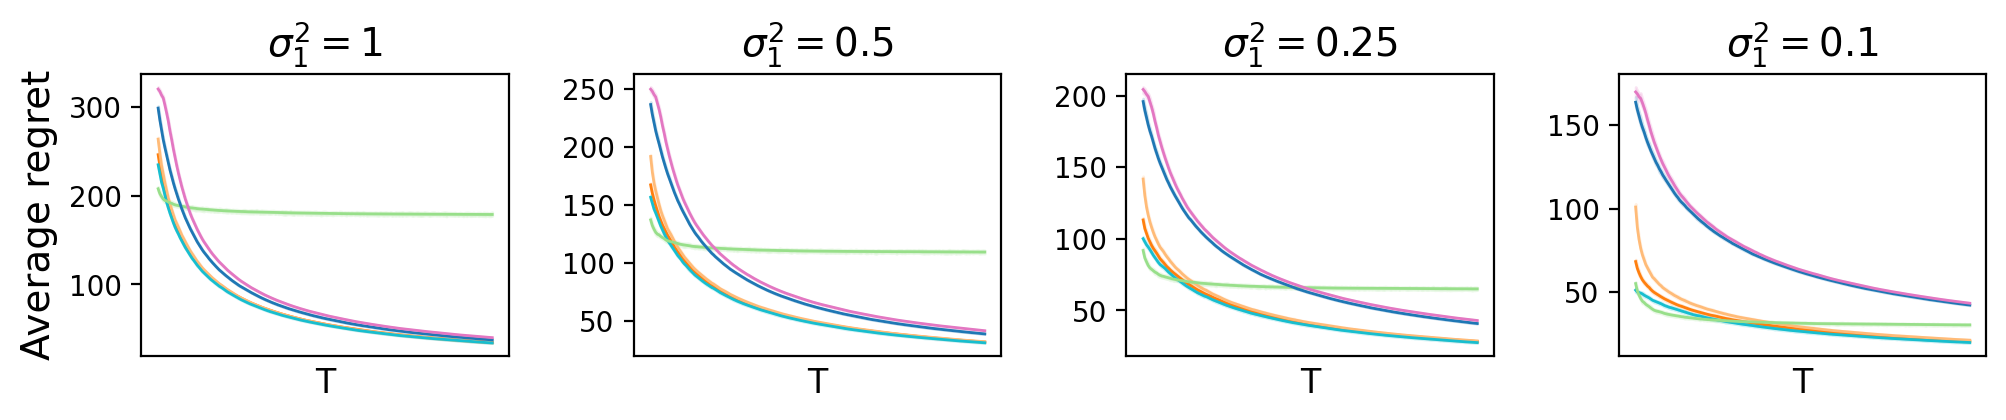}
         \caption{$\lambda = 3/4$}
     \end{subfigure}
     \\
     \begin{subfigure}[b]{\textwidth}
         \centering
         \includegraphics[width=\textwidth]{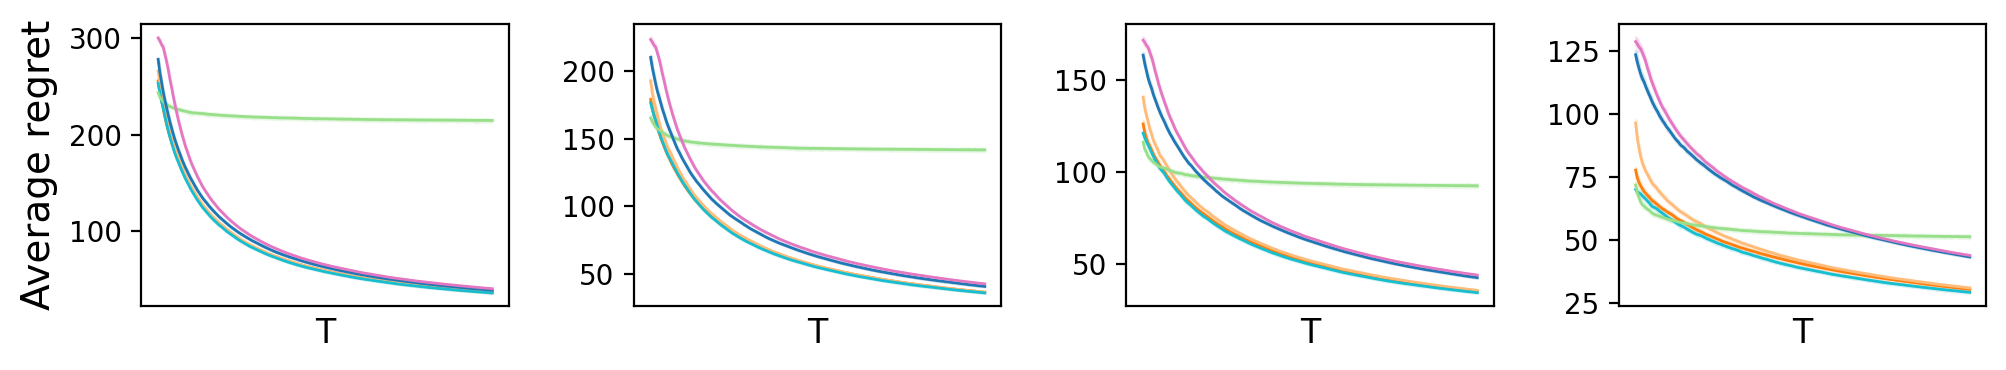}
         \caption{$\lambda = 1/2$}
     \end{subfigure}
     \\
     \begin{subfigure}[b]{\textwidth}
         \centering
         \includegraphics[width=\textwidth]{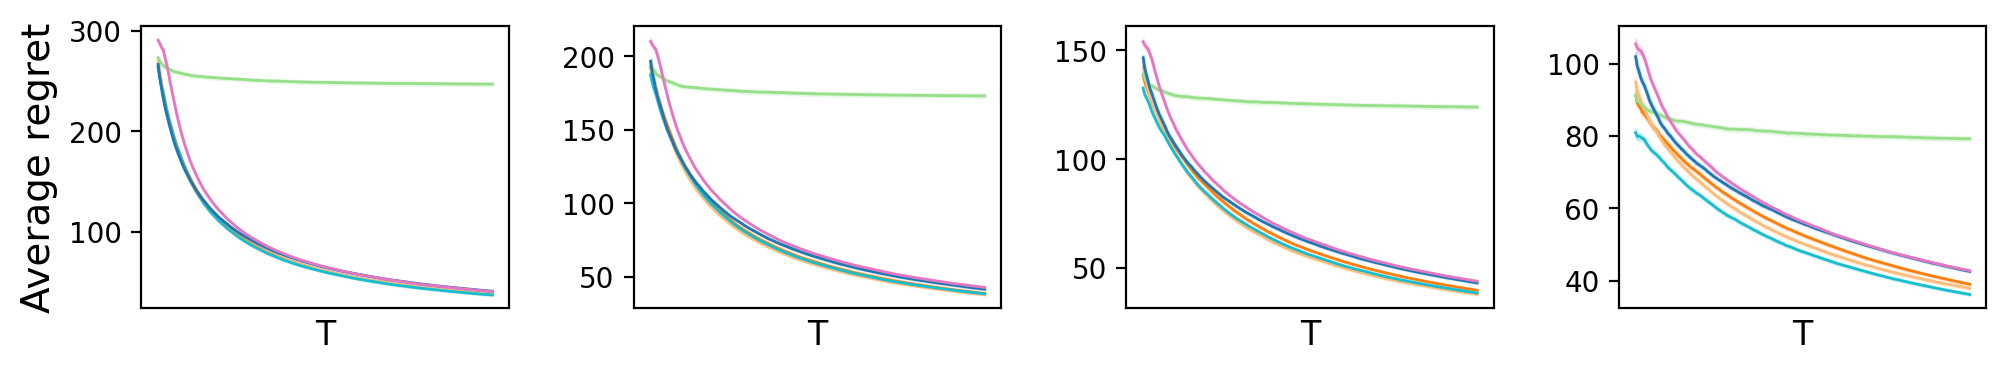}
         \caption{$\lambda = 1/4$}
     \end{subfigure}
     \\
     \begin{subfigure}[b]{\textwidth}
         \centering
         \includegraphics[width=\textwidth]{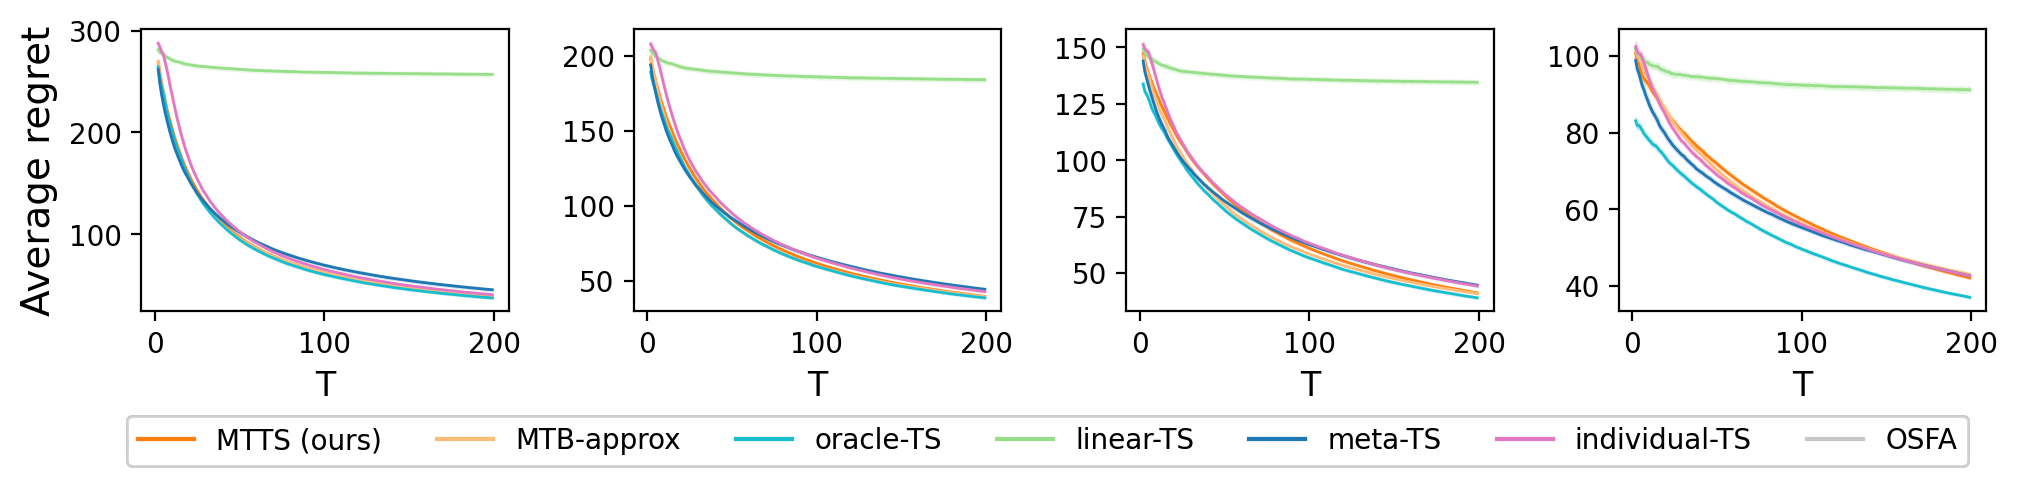}
         \caption{$\lambda = 0$}
     \end{subfigure}
     \\
\caption{
Average Bayes regret for Gaussian bandits with misspecified hierarchical models. 
A smaller value of $\lambda$ implies a more severe misspecification. 
The regrets of OSFA are an order of magnitude higher and hence hidden. 
}
% The yellow line (TR, m = 2) and green line (TR, m = 3) are largely overlapped
\label{fig:simu_Gaussian_robustness_concurrent}
\end{figure}

% \begin{figure}[t]
%      \centering
%      \begin{subfigure}[b]{\textwidth}
%          \centering
%          \includegraphics[width=\textwidth]{Figures/mis_cos_0_1_episodic.png}
%          \caption{$\lambda = 0$}
%      \end{subfigure}
%      \\
%      \begin{subfigure}[b]{\textwidth}
%          \centering
%          \includegraphics[width=\textwidth]{Figures/mis_cos_0.25_0.75_episodic.png}
%          \caption{$\lambda = 1/4$}
%      \end{subfigure}
%      \\
%      \begin{subfigure}[b]{\textwidth}
%          \centering
%          \includegraphics[width=\textwidth]{Figures/mis_cos_0.5_0.5_episodic.png}
%          \caption{$\lambda = 1/2$}
%      \end{subfigure}
%      \\
%      \begin{subfigure}[b]{\textwidth}
%          \centering
%          \includegraphics[width=\textwidth]{Figures/mis_cos_0.75_0.25_episodic.png}
%          \caption{$\lambda = 3/4$}
%      \end{subfigure}
%      \\
% \caption{
% Average Bayes regret for Gaussian bandits with misspecified hierarchical models. 
% A smaller value of $\lambda$ implies a more serious misspecification. 
% The regrets of OSFA are an order of magnitude higher and hence hidden in the upper subplots. 
% }
% % The yellow line (TR, m = 2) and green line (TR, m = 3) are largely overlapped
% \label{fig:simu_Gaussian_robustness_concurrent}
% \end{figure}

\subsection{Multi-task regrets}\label{sec:appendix_figure_MTR}
In the main text, we report the Bayes regret of different algorithms. 
Although the multi-task regrets for those figures can also be derived according to its definition, we choose to explicitly report them again in this section, in order to make the comparison more clearly. 

Specifically, the multi-task regrets for Gaussian bandits and Bernoulli bandits are presented in Figure \ref{fig:simu_Gaussian_multi-task}  and \ref{fig:simu_Binary_multi-task}, respectively. 
In the sequential setting, we can see the multi-task regrets of {\name} converge to zero, while meta-TS and individual-TS have a constant regret, and linear-TS as well as OSFA suffer from the bias.

\begin{figure}[h]
     \centering
 \begin{subfigure}[b]{\textwidth}
     \centering
     \includegraphics[width=\textwidth]{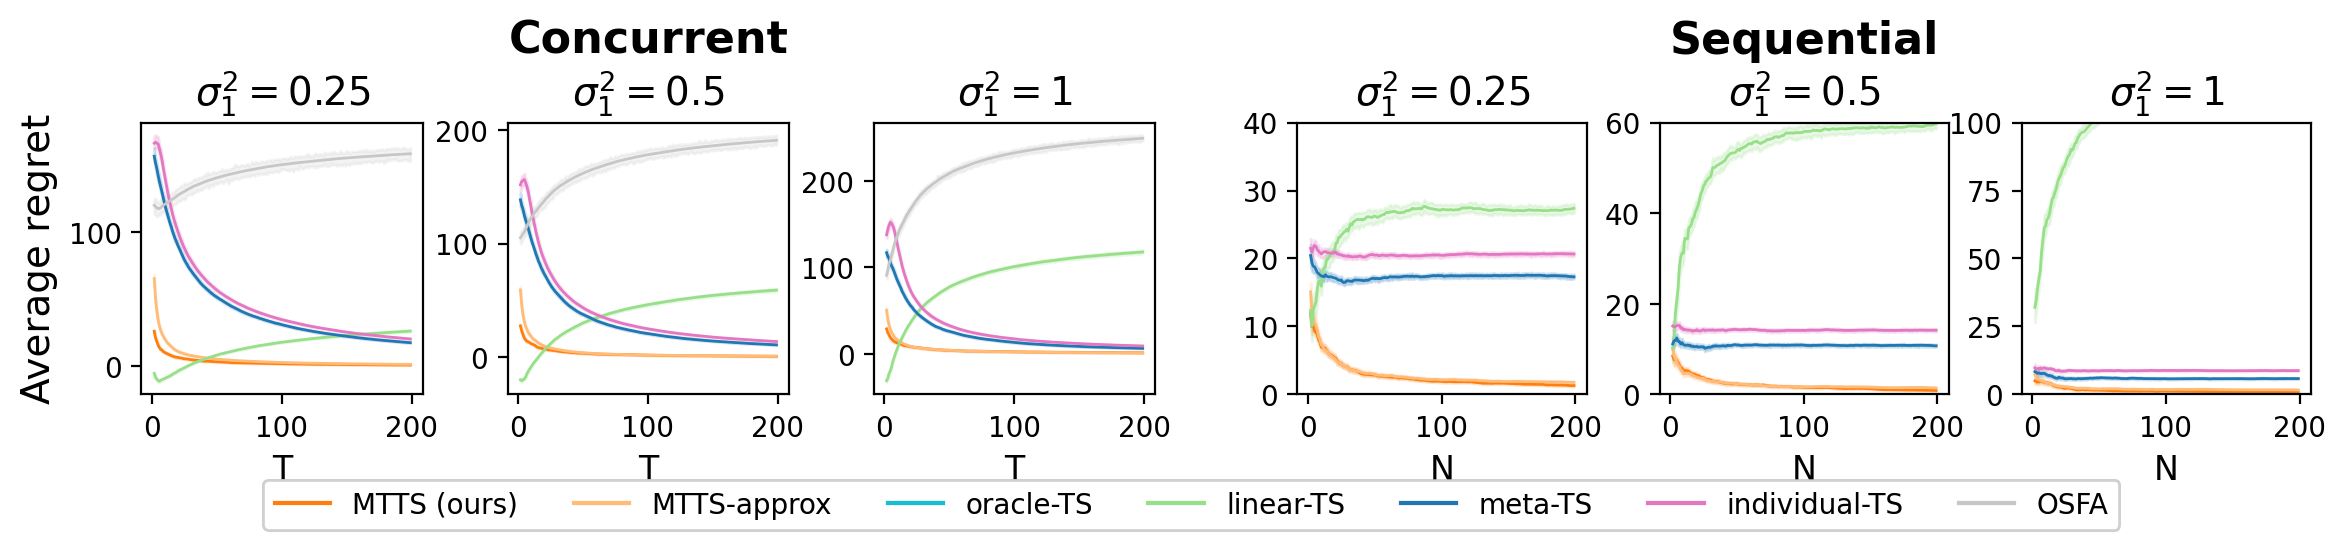}
    %  \caption{Episodic, $\sigma_3 = 5$}
    %  \label{fig:y equals x}
 \end{subfigure}
\caption{
Gaussian bandits: 
the solid lines denote the average multi-task regret with the shared areas indicating the standard errors.  
The regrets of OSFA are much higher in some subplots and hence hidden.
}
% an order of magnitude
% The yellow line (TR, m = 2) and green line (TR, m = 3) are largely overlapped
\label{fig:simu_Gaussian_multi-task}
\end{figure}
\begin{figure}[h]
 \centering
 \begin{subfigure}[b]{\textwidth}
     \centering
     \includegraphics[width=\textwidth]{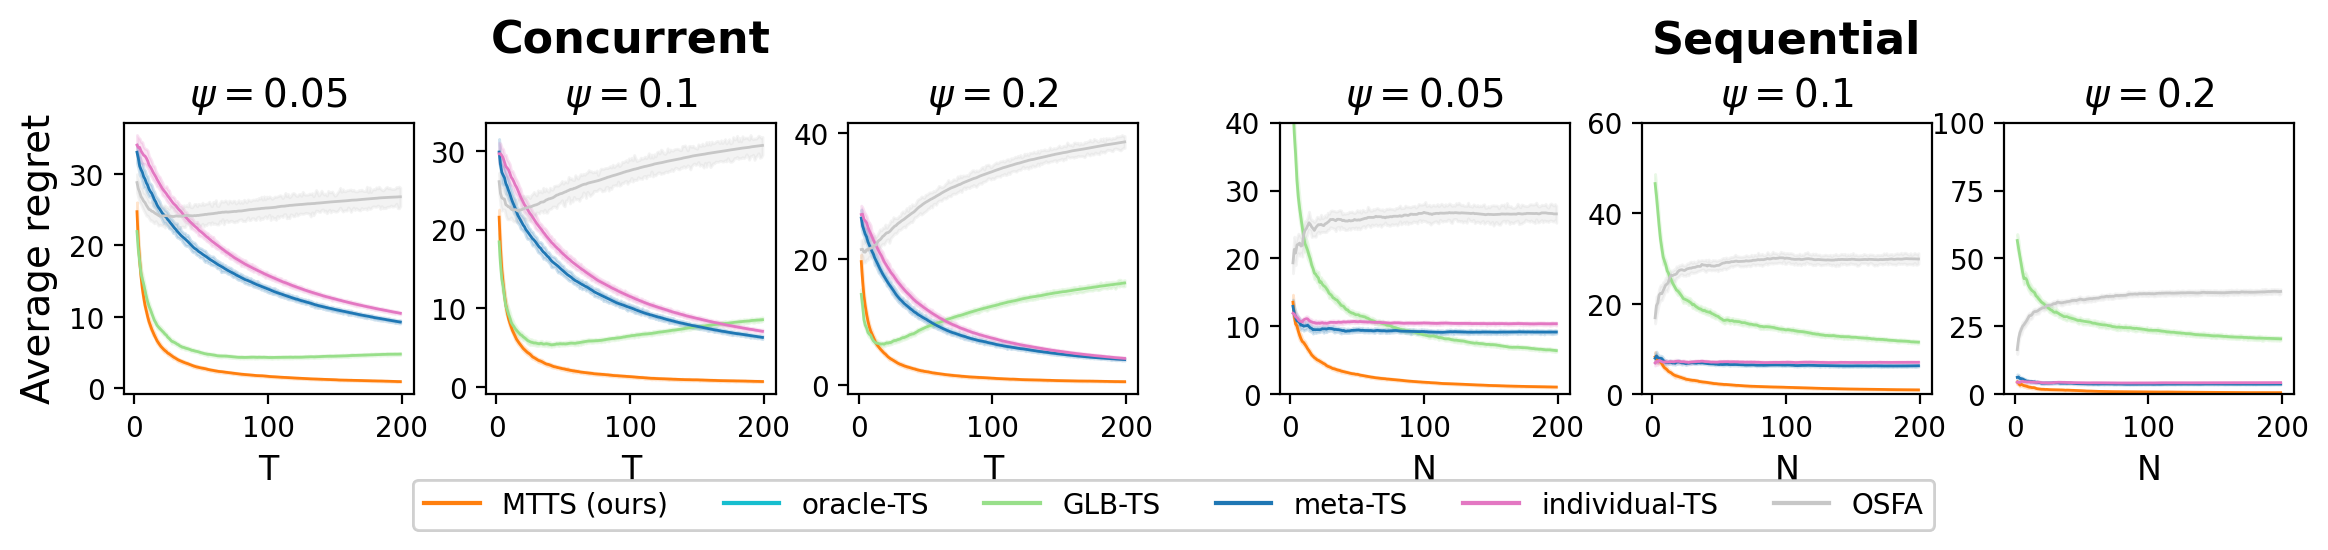}
    %  \caption{Episodic, $\sigma_3 = 5$}
    %  \label{fig:y equals x}
 \end{subfigure}
\caption{
Bernoulli bandits: 
the solid lines denote the average multi-task regret with the shared areas indicating the standard errors.  
A larger value of $\psi$ implies a larger variation of $\vr_i$ condition on $\vx_i$. 
}
\vspace{-0.3cm}
\label{fig:simu_Binary_multi-task}
\end{figure}

\subsection{Trends with experiment hyper-parameters}\label{sec:appendix_more}
In this section, we report additional results under other combinations of $(K, d, T, N)$, to show that our conclusions in the main text are representative, and study the trend of the performance of {\name}. 
We focus on the Gaussian bandits case under the concurrent setting. 
To save computational cost, we set the base combination of hyper-parameters as $\sigma_1^2 = 0.5$, $K = 8$, $d = 15$, $N = 100$, and $T = 100$, and run $50$ random seeds for each. 

In Figure \ref{fig:simu_Gaussian_trend}, we vary the value of $K$, $d$, $N$, $\sigma$ individually. 
Overall, {\name} consistently demonstrates lower regrets and shows robustness. 
Our findings can be summarized as follows. 
\begin{itemize}
    % we also share information across arms... it is like cheating...
    \item As $K$ increases, the learning problem for all algorithm becomes more difficult. {\name} still demonstrates better performance, and even when $T = 100$, its advantage is still fairly clear.
    \item As $d$ increases, the learning problem for {\name} becomes more difficult, while it still shows much better performance. 
    \item As $\sigma$ increases, overall the learning problem for all algorithm becomes more difficult. {\name} still demonstrates better performance, and even when $T = 100$, its advantage is still fairly clear.
    \item As $N$ increases, {\name} can learn the task distribution more easily and its performance converges to that of oracle-TS more quickly. 
\end{itemize}

\begin{figure}[h]
     \centering
     \begin{subfigure}[b]{\textwidth}
         \centering
         \includegraphics[width=\textwidth]{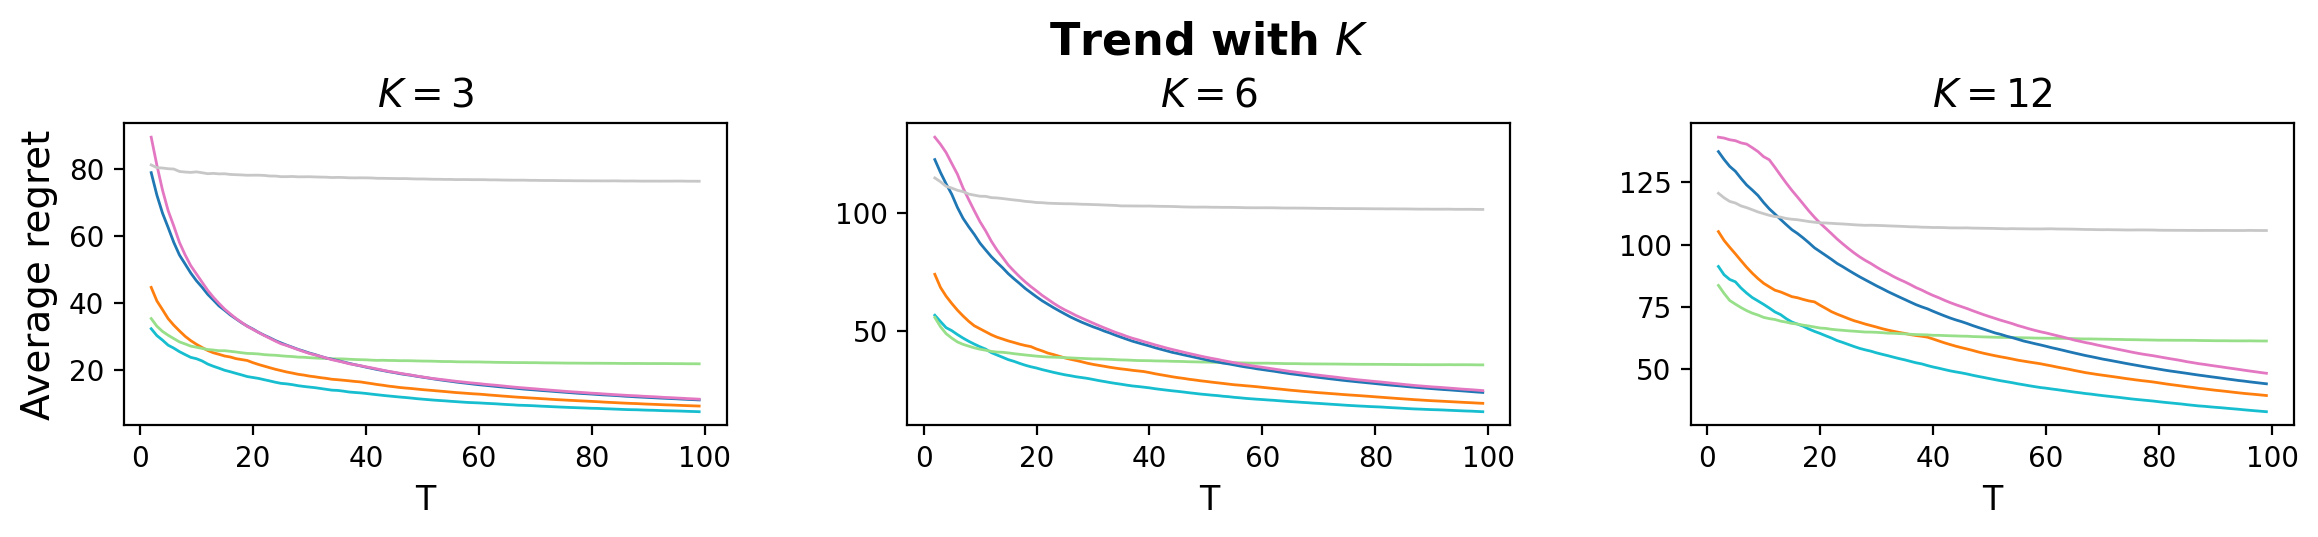}
        %  \caption{$\lambda = 3/4$}
     \end{subfigure}
     \\
     \begin{subfigure}[b]{\textwidth}
         \centering
         \includegraphics[width=\textwidth]{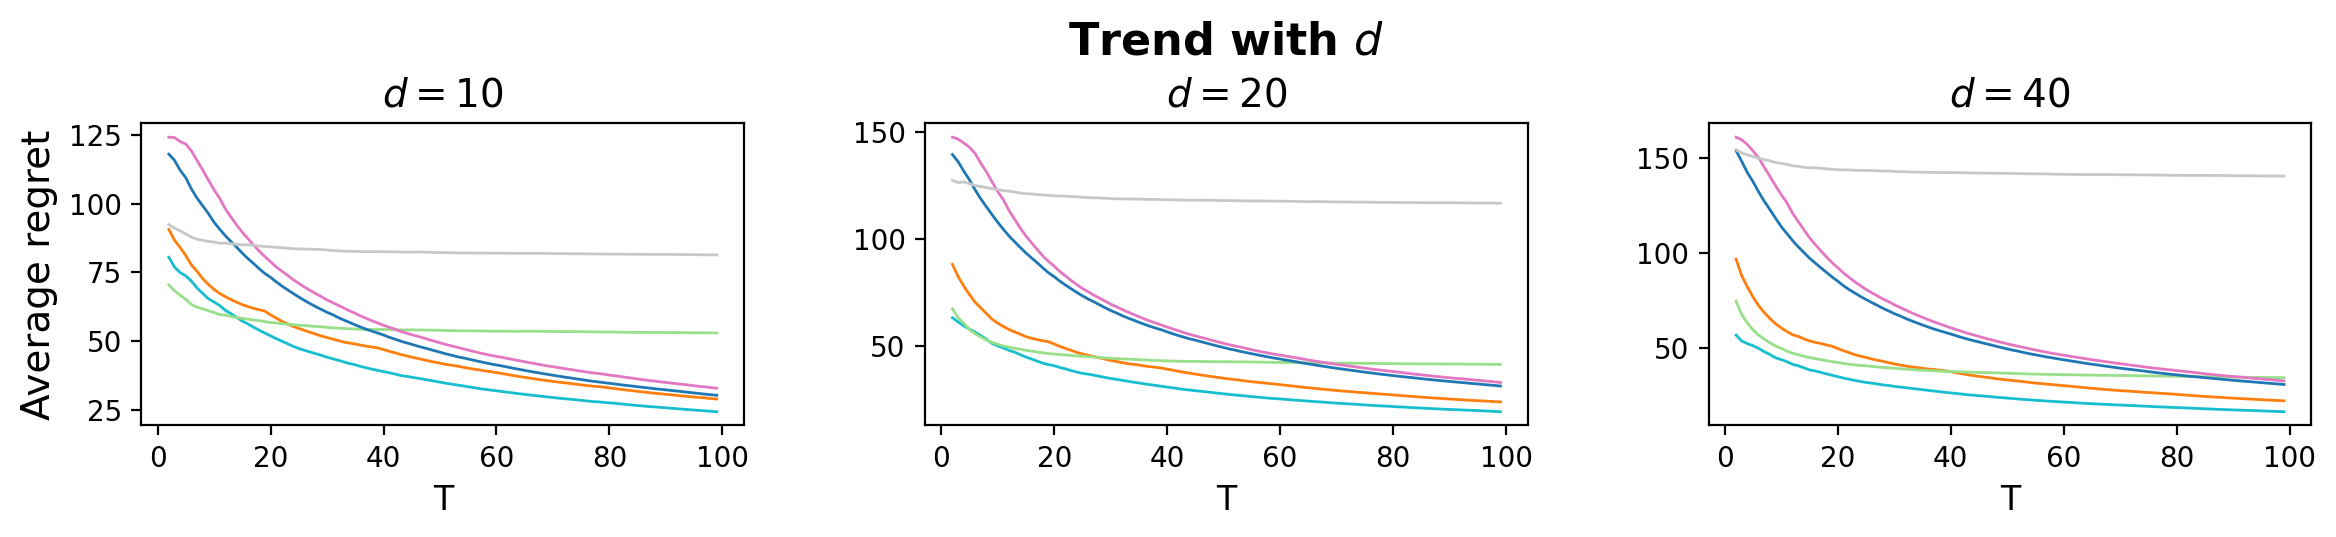}
        %  \caption{$\lambda = 1/4$}
     \end{subfigure}
     \\
     \begin{subfigure}[b]{\textwidth}
         \centering
         \includegraphics[width=\textwidth]{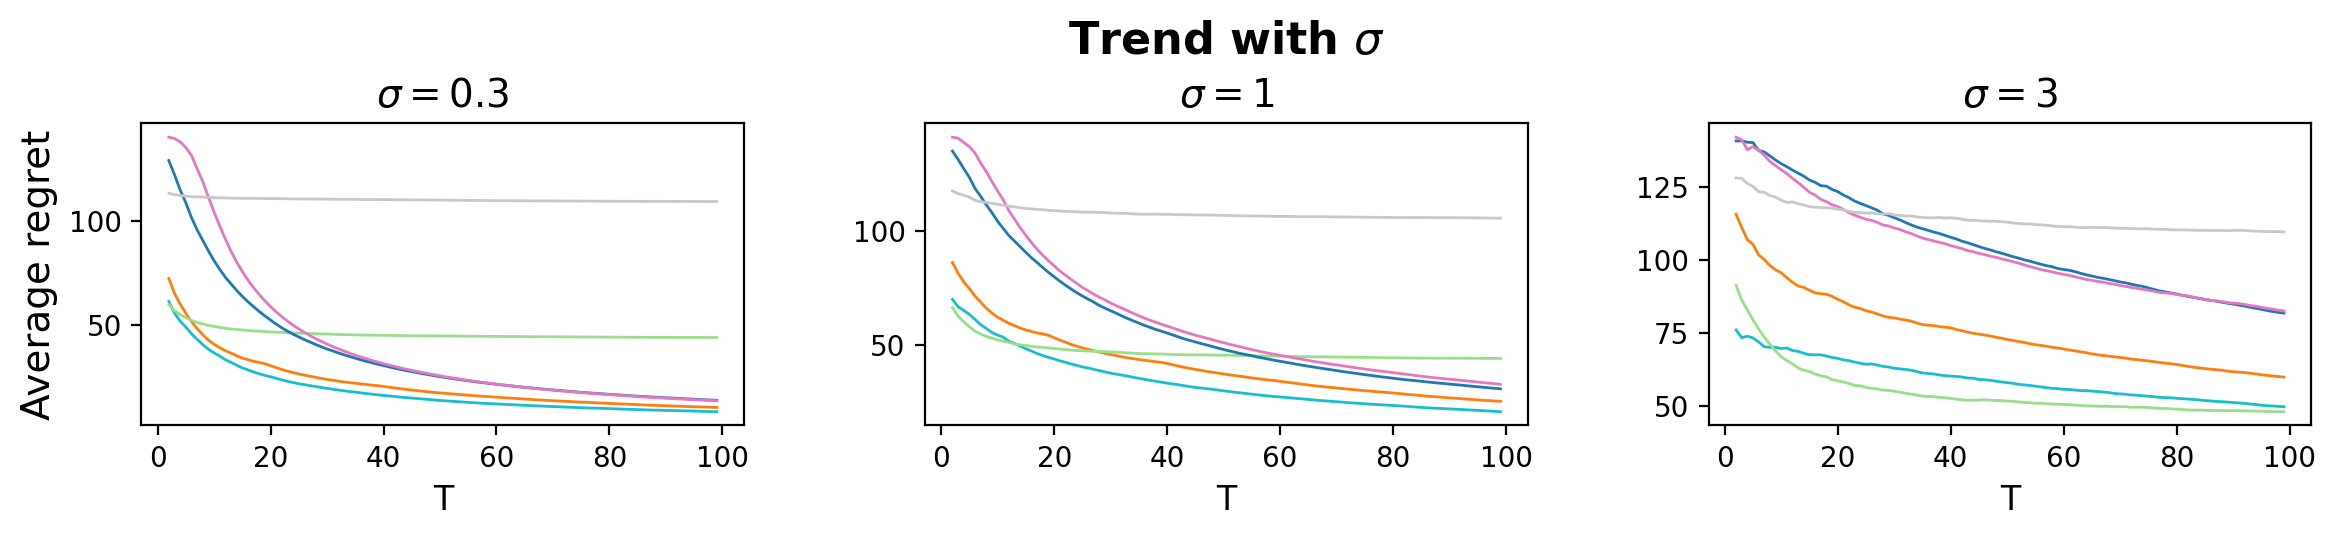}
        %  \caption{$\lambda = 0$}
     \end{subfigure}
     \\
     \begin{subfigure}[b]{\textwidth}
         \centering
         \includegraphics[width=\textwidth]{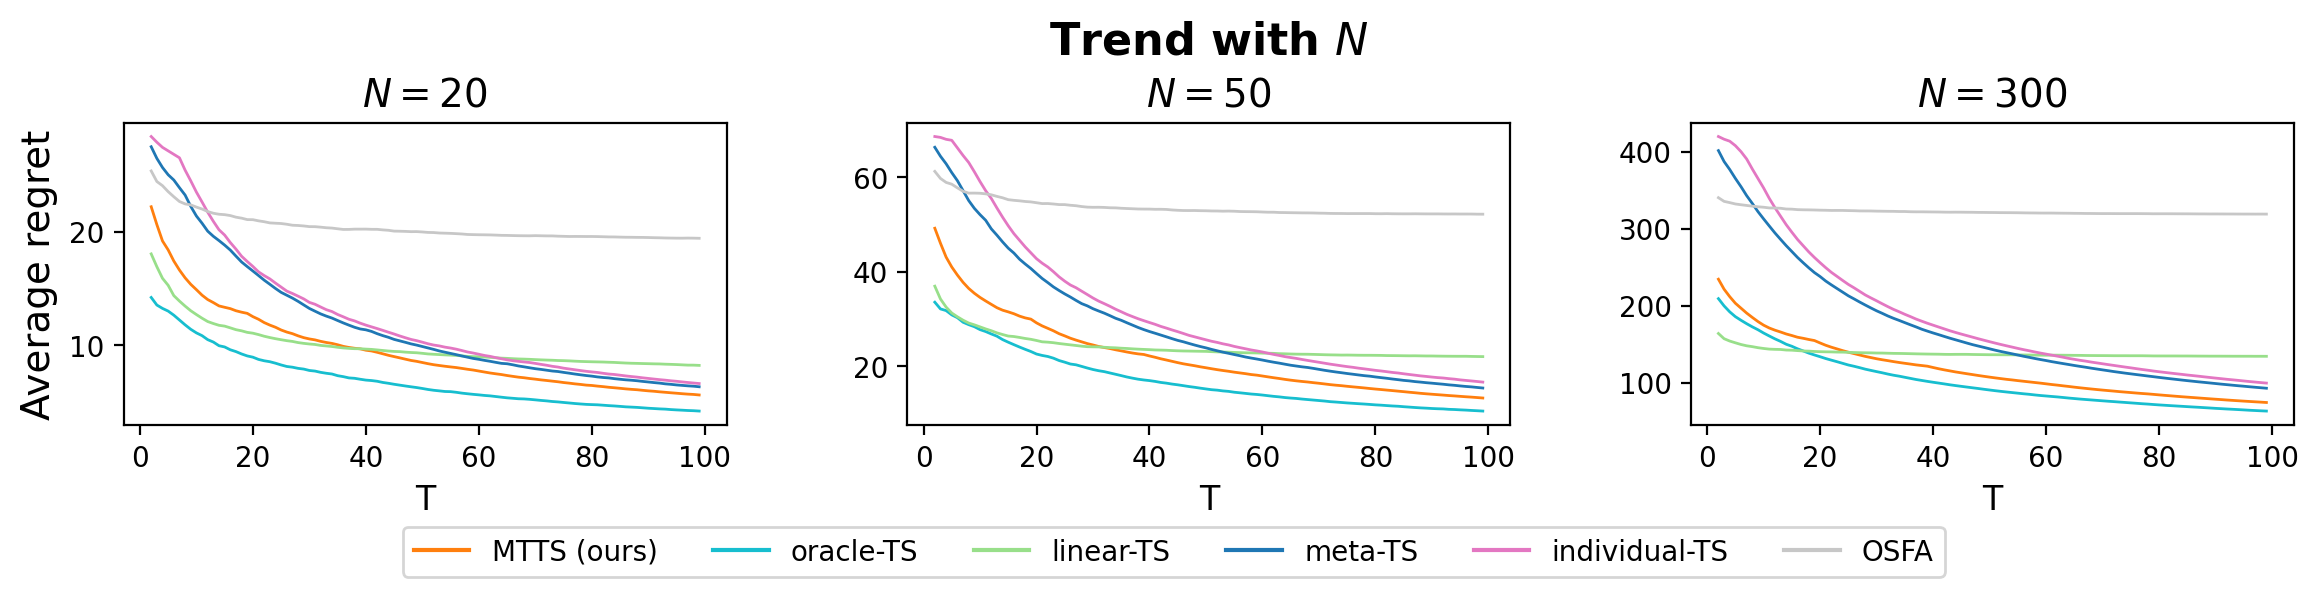}
        %  \caption{$\lambda = 1/2$}
     \end{subfigure}
     \\
\caption{
Trends of the average Bayes regret for Gaussian bandits with different parameters. 
% under different settings. . 
}
% The yellow line (TR, m = 2) and green line (TR, m = 3) are largely overlapped
\label{fig:simu_Gaussian_trend}
\end{figure}
